# Supplementary material for: Drug cell line interaction prediction
Source: arXiv:1812.11178 source file (2018-12-28)
Supplement: Supplementary file 1 [file Supplementary.pdf]

# Supplementary

Improving Prediction of Phenotypic Drug Response on Cancer Cell Lines Using Deep Convolutional Network

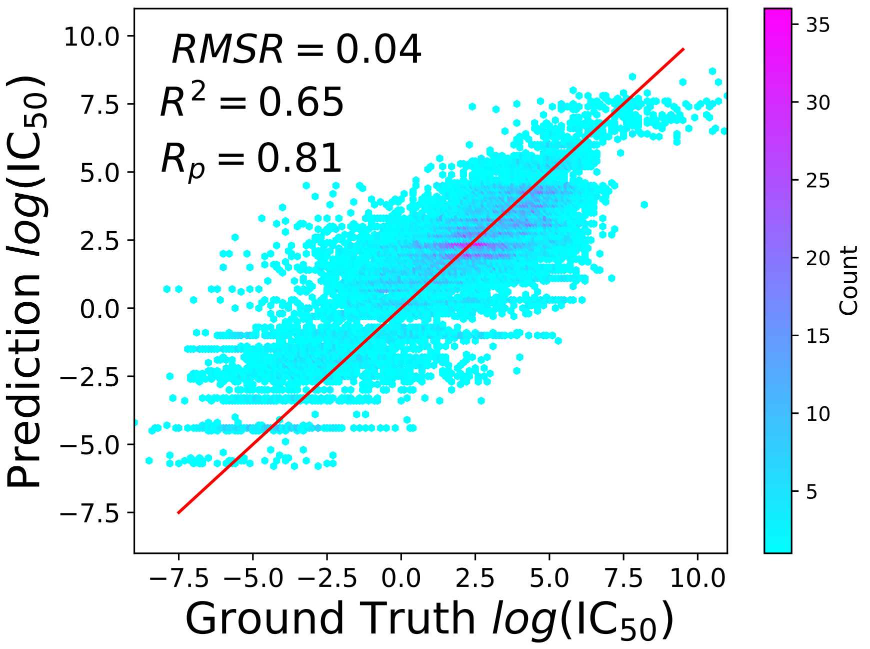


Figure 1: Regression result using PaDEL features for the drugs. We can see that the result is horizontally stratified, which indicates the lack of representation power for the network.

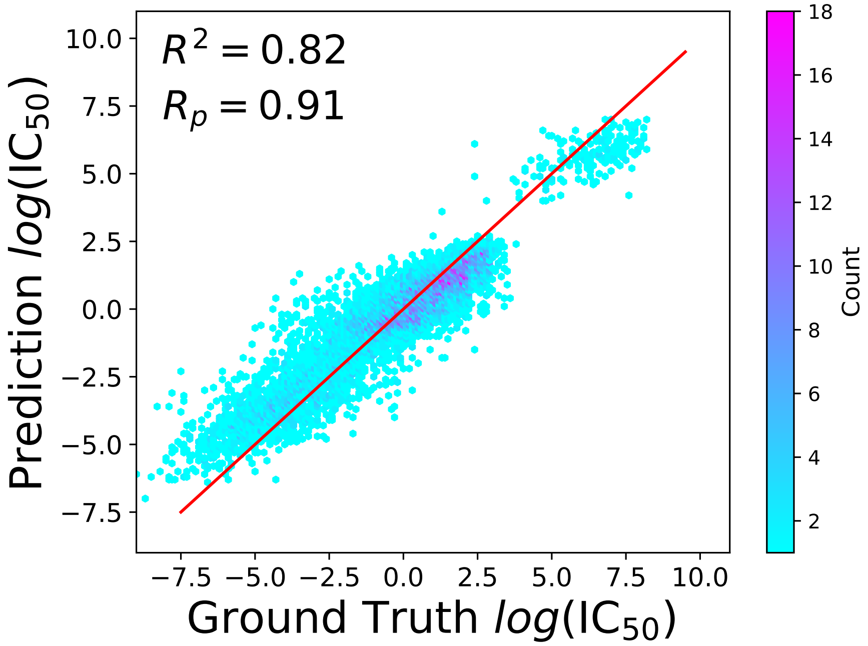


Figure 2: Regression result for max_conc data. $R^2$ and $R_p$ are similar to the main result of the paper. The data below max_conc are not uniformly distributed, and they formed two distinguished groups.

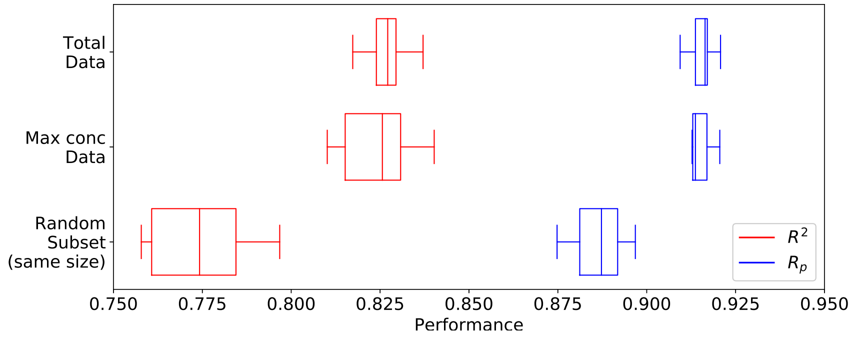


Figure 3: Influence of data quantity and quality. The first row is the result on all existing data ($172,114$ $\mathrm{IC}_{50}$ values), and the second row is the result on data below max_conc threshold ($64,440$ $\mathrm{IC}_{50}$ values), and the third row is the result on a random subset of all data with the same size as those below the max_conc threshold ($64,440$).

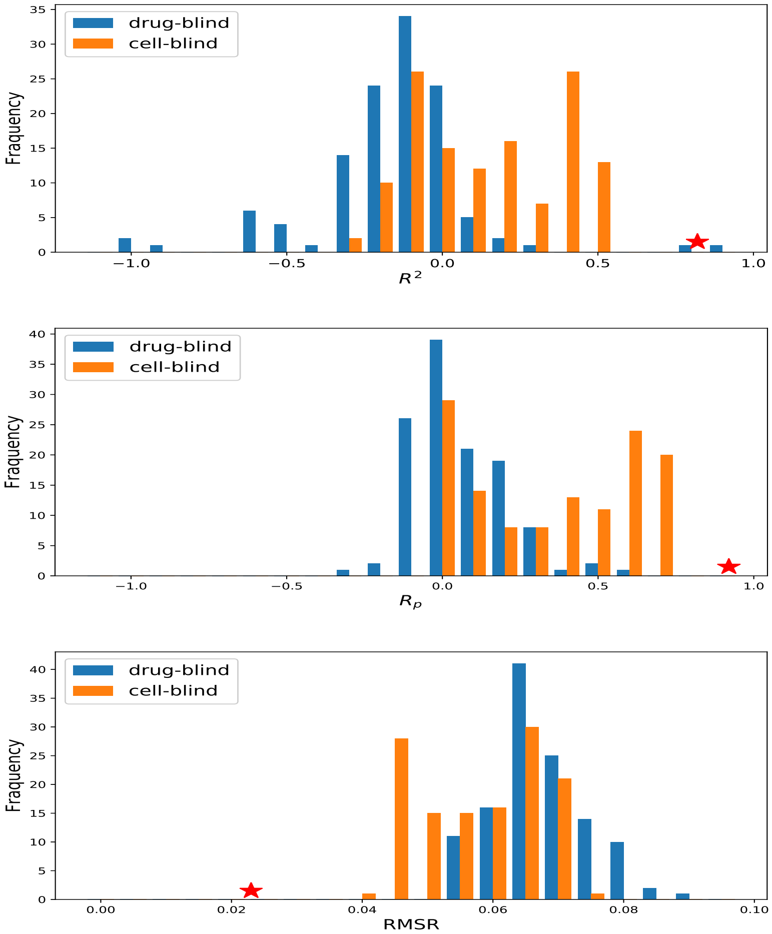


Figure 4: The blind test results for drugs and cell lines on data below the max_conc threshold. The yellow color boxes represent the result of cell lines, and the blue color boxes represent the result for drugs. From up to down is the result for $R^2$, $R_p$ and $RMSR$ respectively. The red stars are the results in normal experiments.

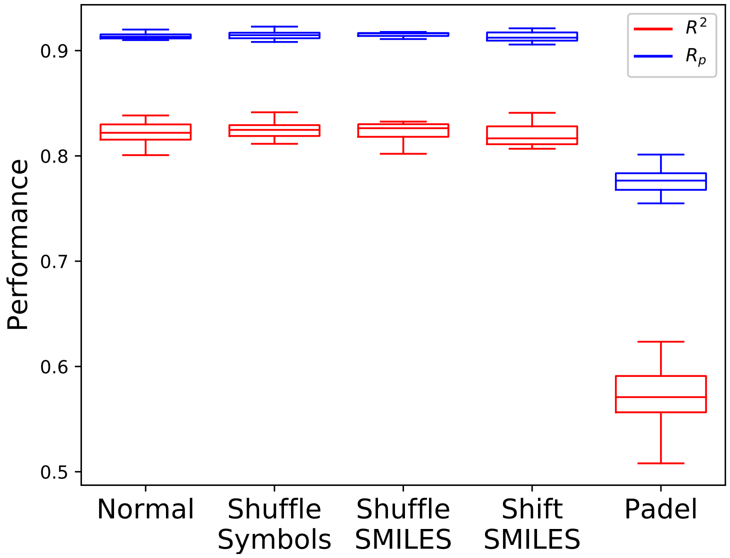


Figure 5: Performance of different ways to modify the input data. The first column is the original setting we use. The second column is the result by shuffle the order of symbols, the third column is the result by shuffle the SMILES, the fourth column is the result by shifting the SMILES. The last column is the result using the PaDEL features for drugs, just like the setting in the benchmark.

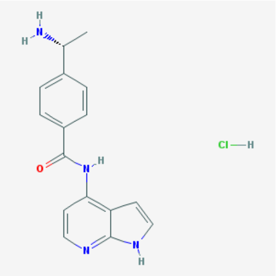

Y-39983

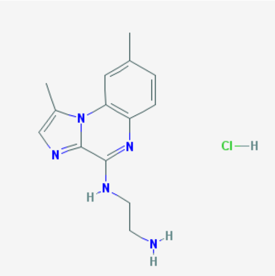

BMS-345541

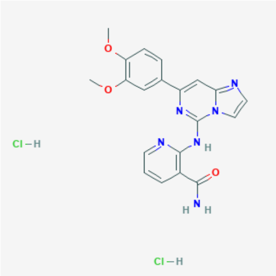

BAY-61-3606

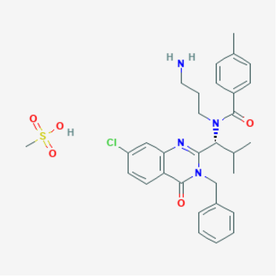

Ispinesib
Mesylate

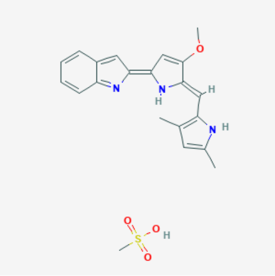

Obatoclax
Mesylate

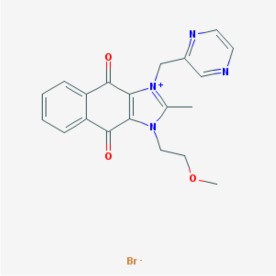

Sepantronium
bromide

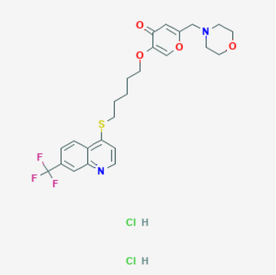

EHT-1864

Figure 6: The seven outliers in PaDEL's feature space for drugs.
